# Supplementary material for: On Evaluating the Renaissance Benchmarking Suite: Variety, Performance, and Complexity
Source: arXiv:1903.10267 source file (2019-03-25)
Supplement: Supplementary file 2 [file table-appendix.tex]

\begin{tabular}{l | rrrrrrrrrrr}
\hline
{\bf Benchmark}&\metric{\bf synch}&\metric{\bf wait}&\metric{\bf notify}&\metric{\bf atomic}&\metric{\bf park}&\metric{\bf cpu}&\metric{\bf cachemiss}&\metric{\bf object}&\metric{\bf array}&\metric{\bf method}&\metric{\bf idynamic}\\
\hline
\multicolumn{12}{c}{\bf Renaissance}\\
\hline
\bench{akka-uct}&{\tt 4.46E-07}&{\tt 1.04E-12}&{\tt 2.09E-12}&{\tt 1.24E-05}&{\tt 1.83E-07}&{\tt 94.45}&{\tt 3.36E-02}&{\tt 2.04E-05}&{\tt 1.05E-07}&{\tt 3.43E-04}&{\tt 0.00E+00}\\\hdashline[0.5pt/1pt]
\bench{als}&{\tt 2.27E-05}&{\tt 8.68E-10}&{\tt 9.87E-08}&{\tt 1.36E-05}&{\tt 1.81E-08}&{\tt 58.90}&{\tt 1.21E-02}&{\tt 1.08E-05}&{\tt 2.33E-06}&{\tt 2.85E-04}&{\tt 0.00E+00}\\\hdashline[0.5pt/1pt]
\bench{chi-square}&{\tt 3.28E-05}&{\tt 1.87E-09}&{\tt 9.26E-10}&{\tt 3.41E-06}&{\tt 1.55E-09}&{\tt 26.19}&{\tt 3.67E-02}&{\tt 2.30E-05}&{\tt 3.20E-06}&{\tt 3.19E-04}&{\tt 0.00E+00}\\\hdashline[0.5pt/1pt]
\bench{dec-tree}&{\tt 1.03E-05}&{\tt 1.55E-09}&{\tt 2.42E-08}&{\tt 9.62E-06}&{\tt 9.45E-09}&{\tt 27.23}&{\tt 3.97E-02}&{\tt 2.57E-05}&{\tt 2.92E-06}&{\tt 3.04E-04}&{\tt 0.00E+00}\\\hdashline[0.5pt/1pt]
\bench{db-shootout}&{\tt 2.95E-05}&{\tt 1.30E-10}&{\tt 0.00E+00}&{\tt 1.10E-04}&{\tt 1.63E-06}&{\tt 45.53}&{\tt 3.59E-02}&{\tt 8.77E-06}&{\tt 7.80E-06}&{\tt 4.51E-04}&{\tt 4.05E-08}\\\hdashline[0.5pt/1pt]
\bench{dotty}&{\tt 8.13E-05}&{\tt 5.77E-11}&{\tt 3.70E-07}&{\tt 6.25E-07}&{\tt 0.00E+00}&{\tt 15.68}&{\tt 4.02E-02}&{\tt 6.06E-05}&{\tt 1.75E-05}&{\tt 1.55E-03}&{\tt 8.91E-06}\\\hdashline[0.5pt/1pt]
\bench{finagle-chirper}&{\tt 4.55E-05}&{\tt 6.05E-09}&{\tt 6.13E-09}&{\tt 3.60E-04}&{\tt 6.03E-08}&{\tt 69.82}&{\tt 4.58E-02}&{\tt 7.18E-06}&{\tt 5.06E-07}&{\tt 2.22E-04}&{\tt 1.18E-10}\\\hdashline[0.5pt/1pt]
\bench{finagle-http}&{\tt 1.10E-07}&{\tt 8.08E-11}&{\tt 0.00E+00}&{\tt 2.10E-07}&{\tt 2.69E-09}&{\tt 14.72}&{\tt 3.52E-02}&{\tt 2.08E-04}&{\tt 4.73E-08}&{\tt 2.29E-03}&{\tt 4.29E-10}\\\hdashline[0.5pt/1pt]
\bench{fj-kmeans}&{\tt 2.27E-03}&{\tt 1.48E-08}&{\tt 1.49E-08}&{\tt 4.26E-07}&{\tt 2.67E-08}&{\tt 69.59}&{\tt 3.82E-03}&{\tt 6.33E-05}&{\tt 1.15E-09}&{\tt 3.34E-04}&{\tt 0.00E+00}\\\hdashline[0.5pt/1pt]
\bench{future-genetic}&{\tt 1.50E-05}&{\tt 5.31E-07}&{\tt 5.36E-07}&{\tt 1.12E-03}&{\tt 3.55E-06}&{\tt 55.85}&{\tt 4.09E-02}&{\tt 5.23E-05}&{\tt 6.53E-08}&{\tt 3.92E-04}&{\tt 5.79E-07}\\\hdashline[0.5pt/1pt]
\bench{log-regression}&{\tt 3.66E-06}&{\tt 1.91E-09}&{\tt 1.72E-08}&{\tt 8.36E-06}&{\tt 1.16E-08}&{\tt 24.83}&{\tt 3.55E-02}&{\tt 1.46E-05}&{\tt 4.56E-06}&{\tt 5.06E-04}&{\tt 0.00E+00}\\\hdashline[0.5pt/1pt]
\bench{movie-lens}&{\tt 3.96E-05}&{\tt 1.85E-09}&{\tt 7.11E-07}&{\tt 9.95E-05}&{\tt 1.27E-07}&{\tt 44.17}&{\tt 3.36E-02}&{\tt 8.32E-06}&{\tt 1.07E-06}&{\tt 3.04E-04}&{\tt 8.96E-12}\\\hdashline[0.5pt/1pt]
\bench{naive-bayes}&{\tt 4.07E-06}&{\tt 6.13E-10}&{\tt 1.91E-09}&{\tt 3.17E-07}&{\tt 2.31E-09}&{\tt 76.90}&{\tt 4.12E-02}&{\tt 2.31E-05}&{\tt 5.25E-06}&{\tt 2.34E-04}&{\tt 0.00E+00}\\\hdashline[0.5pt/1pt]
\bench{neo4j-analytics}&{\tt 4.16E-05}&{\tt 1.29E-09}&{\tt 4.69E-07}&{\tt 6.24E-06}&{\tt 6.14E-10}&{\tt 59.74}&{\tt 9.38E+06}&{\tt 8.97E-06}&{\tt 2.08E-07}&{\tt 1.40E-04}&{\tt 1.57E-07}\\\hdashline[0.5pt/1pt]
\bench{page-rank}&{\tt 2.73E-05}&{\tt 9.44E-10}&{\tt 1.31E-09}&{\tt 9.59E-05}&{\tt 1.43E-09}&{\tt 56.14}&{\tt 2.68E-02}&{\tt 1.03E-05}&{\tt 1.50E-07}&{\tt 2.62E-04}&{\tt 0.00E+00}\\\hdashline[0.5pt/1pt]
\bench{philosophers}&{\tt 1.19E-05}&{\tt 8.18E-08}&{\tt 4.39E-07}&{\tt 6.36E-04}&{\tt 1.36E-07}&{\tt 99.21}&{\tt 2.36E-02}&{\tt 5.41E-06}&{\tt 1.44E-06}&{\tt 1.89E-04}&{\tt 0.00E+00}\\\hdashline[0.5pt/1pt]
\bench{reactors}&{\tt 1.13E-04}&{\tt 0.00E+00}&{\tt 0.00E+00}&{\tt 7.66E-05}&{\tt 2.40E-06}&{\tt 56.62}&{\tt 1.26E-02}&{\tt 7.71E-06}&{\tt 5.29E-07}&{\tt 3.54E-04}&{\tt 0.00E+00}\\\hdashline[0.5pt/1pt]
\bench{rx-scrabble}&{\tt 1.33E-04}&{\tt 0.00E+00}&{\tt 0.00E+00}&{\tt 1.32E-05}&{\tt 1.56E-09}&{\tt 25.10}&{\tt 2.30E-02}&{\tt 8.14E-05}&{\tt 0.00E+00}&{\tt 7.77E-04}&{\tt 1.30E-05}\\\hdashline[0.5pt/1pt]
\bench{stm-bench7}&{\tt 2.06E-07}&{\tt 5.78E-10}&{\tt 1.73E-10}&{\tt 1.69E-04}&{\tt 0.00E+00}&{\tt 49.44}&{\tt 2.80E-02}&{\tt 1.95E-05}&{\tt 1.90E-06}&{\tt 5.24E-04}&{\tt 0.00E+00}\\\hdashline[0.5pt/1pt]
\bench{scrabble}&{\tt 1.24E-10}&{\tt 6.18E-11}&{\tt 6.18E-11}&{\tt 1.85E-09}&{\tt 6.18E-11}&{\tt 66.70}&{\tt 4.46E-02}&{\tt 2.60E-05}&{\tt 1.59E-06}&{\tt 2.30E-04}&{\tt 1.26E-05}\\\hdashline[0.5pt/1pt]
\bench{streams-mnemonics}&{\tt 0.00E+00}&{\tt 0.00E+00}&{\tt 0.00E+00}&{\tt 0.00E+00}&{\tt 0.00E+00}&{\tt 19.24}&{\tt 5.18E-02}&{\tt 3.19E-04}&{\tt 3.28E-04}&{\tt 1.80E-03}&{\tt 3.36E-05}\\
\hline
\multicolumn{12}{c}{\bf DaCapo~\cite{Blackburn:2006:DBJ:1167515.1167488}}\\
\hline
\bench{avrora}&{\tt 3.26E-05}&{\tt 7.89E-06}&{\tt 7.61E-07}&{\tt 0.00E+00}&{\tt 0.00E+00}&{\tt 20.28}&{\tt 1.06E+07}&{\tt 1.10E-06}&{\tt 3.12E-07}&{\tt 4.23E-04}&{\tt 0.00E+00}\\\hdashline[0.5pt/1pt]
\bench{batik}&{\tt 8.56E-05}&{\tt 3.08E-10}&{\tt 0.00E+00}&{\tt 3.59E-10}&{\tt 0.00E+00}&{\tt 24.54}&{\tt 1.96E-02}&{\tt 1.57E-05}&{\tt 3.63E-06}&{\tt 6.19E-04}&{\tt 0.00E+00}\\\hdashline[0.5pt/1pt]
\bench{eclipse}&{\tt 2.26E-05}&{\tt 6.22E-09}&{\tt 1.19E-07}&{\tt 4.23E-08}&{\tt 0.00E+00}&{\tt 13.91}&{\tt 3.30E-02}&{\tt 3.60E-05}&{\tt 3.93E-05}&{\tt 9.59E-04}&{\tt 0.00E+00}\\\hdashline[0.5pt/1pt]
\bench{fop}&{\tt 1.90E-04}&{\tt 0.00E+00}&{\tt 0.00E+00}&{\tt 1.24E-09}&{\tt 0.00E+00}&{\tt 6.25}&{\tt 3.86E-02}&{\tt 1.01E-04}&{\tt 4.39E-05}&{\tt 2.16E-03}&{\tt 0.00E+00}\\\hdashline[0.5pt/1pt]
\bench{h2}&{\tt 1.06E-04}&{\tt 6.38E-10}&{\tt 0.00E+00}&{\tt 3.86E-06}&{\tt 0.00E+00}&{\tt 17.78}&{\tt 2.08E-02}&{\tt 1.65E-05}&{\tt 6.96E-06}&{\tt 1.49E-03}&{\tt 0.00E+00}\\\hdashline[0.5pt/1pt]
\bench{jython}&{\tt 2.22E-04}&{\tt 0.00E+00}&{\tt 0.00E+00}&{\tt 3.61E-05}&{\tt 0.00E+00}&{\tt 11.41}&{\tt 2.11E-02}&{\tt 6.48E-05}&{\tt 1.31E-05}&{\tt 1.94E-03}&{\tt 0.00E+00}\\\hdashline[0.5pt/1pt]
\bench{luindex}&{\tt 9.24E-05}&{\tt 3.33E-10}&{\tt 4.15E-07}&{\tt 3.33E-09}&{\tt 0.00E+00}&{\tt 5.57}&{\tt 2.11E-02}&{\tt 5.08E-06}&{\tt 2.34E-06}&{\tt 2.15E-03}&{\tt 0.00E+00}\\\hdashline[0.5pt/1pt]
\bench{lusearch-fix}&{\tt 5.59E-05}&{\tt 1.22E-09}&{\tt 8.00E-09}&{\tt 4.52E-09}&{\tt 0.00E+00}&{\tt 85.00}&{\tt 4.15E-02}&{\tt 7.41E-06}&{\tt 3.30E-06}&{\tt 4.47E-04}&{\tt 0.00E+00}\\\hdashline[0.5pt/1pt]
\bench{pmd}&{\tt 7.78E-05}&{\tt 0.00E+00}&{\tt 8.52E-08}&{\tt 1.18E-07}&{\tt 7.66E-11}&{\tt 22.26}&{\tt 4.21E-02}&{\tt 1.79E-05}&{\tt 4.94E-06}&{\tt 2.99E-04}&{\tt 0.00E+00}\\\hdashline[0.5pt/1pt]
\bench{sunflow}&{\tt 9.81E-10}&{\tt 3.22E-12}&{\tt 0.00E+00}&{\tt 0.00E+00}&{\tt 0.00E+00}&{\tt 79.55}&{\tt 1.42E-02}&{\tt 1.63E-05}&{\tt 4.13E-07}&{\tt 3.99E-04}&{\tt 0.00E+00}\\\hdashline[0.5pt/1pt]
\bench{tomcat}&{\tt 1.14E-04}&{\tt 3.04E-10}&{\tt 1.10E-07}&{\tt 3.94E-06}&{\tt 9.70E-08}&{\tt 27.51}&{\tt 7.84E+06}&{\tt 9.06E-06}&{\tt 6.43E-06}&{\tt 3.75E-04}&{\tt 0.00E+00}\\\hdashline[0.5pt/1pt]
\bench{tradesoap}&{\tt 2.01E-04}&{\tt 5.82E-11}&{\tt 3.54E-07}&{\tt 6.57E-07}&{\tt 3.58E-08}&{\tt 64.92}&{\tt 3.54E-02}&{\tt 8.91E-06}&{\tt 3.28E-06}&{\tt 2.01E-04}&{\tt 1.88E-12}\\\hdashline[0.5pt/1pt]
\bench{xalan}&{\tt 3.69E-04}&{\tt 6.06E-10}&{\tt 1.75E-07}&{\tt 0.00E+00}&{\tt 0.00E+00}&{\tt 97.89}&{\tt 2.27E-02}&{\tt 6.07E-06}&{\tt 3.97E-06}&{\tt 3.81E-04}&{\tt 0.00E+00}\\
\hline
\multicolumn{12}{c}{\bf ScalaBench~\cite{Sewe:2011:DCC:2048066.2048118}}\\
\hline
\bench{apparat}&{\tt 1.45E-05}&{\tt 6.05E-09}&{\tt 5.54E-07}&{\tt 1.28E-06}&{\tt 4.87E-08}&{\tt 15.80}&{\tt 7.10E-02}&{\tt 2.88E-06}&{\tt 2.28E-07}&{\tt 8.97E-04}&{\tt 0.00E+00}\\\hdashline[0.5pt/1pt]
\bench{factorie}&{\tt 2.51E-05}&{\tt 2.42E-12}&{\tt 0.00E+00}&{\tt 7.93E-05}&{\tt 0.00E+00}&{\tt 12.04}&{\tt 3.32E-02}&{\tt 1.78E-04}&{\tt 2.79E-06}&{\tt 1.44E-03}&{\tt 0.00E+00}\\\hdashline[0.5pt/1pt]
\bench{kiama}&{\tt 1.24E-05}&{\tt 0.00E+00}&{\tt 0.00E+00}&{\tt 0.00E+00}&{\tt 0.00E+00}&{\tt 0.00}&{\tt 2.90E-02}&{\tt 1.17E-04}&{\tt 2.53E-05}&{\tt 1.10E-03}&{\tt 0.00E+00}\\\hdashline[0.5pt/1pt]
\bench{scalac}&{\tt 3.60E-05}&{\tt 0.00E+00}&{\tt 0.00E+00}&{\tt 0.00E+00}&{\tt 0.00E+00}&{\tt 15.45}&{\tt 4.43E-02}&{\tt 4.51E-05}&{\tt 6.20E-06}&{\tt 1.22E-03}&{\tt 0.00E+00}\\\hdashline[0.5pt/1pt]
\bench{scaladoc}&{\tt 4.98E-05}&{\tt 0.00E+00}&{\tt 0.00E+00}&{\tt 0.00E+00}&{\tt 0.00E+00}&{\tt 6.11}&{\tt 4.01E-02}&{\tt 5.32E-05}&{\tt 1.03E-05}&{\tt 1.33E-03}&{\tt 0.00E+00}\\\hdashline[0.5pt/1pt]
\bench{scalap}&{\tt 4.50E-05}&{\tt 0.00E+00}&{\tt 0.00E+00}&{\tt 0.00E+00}&{\tt 0.00E+00}&{\tt 0.00}&{\tt 3.62E-02}&{\tt 5.40E-05}&{\tt 5.42E-06}&{\tt 1.23E-03}&{\tt 0.00E+00}\\\hdashline[0.5pt/1pt]
\bench{scalariform}&{\tt 5.96E-05}&{\tt 0.00E+00}&{\tt 0.00E+00}&{\tt 0.00E+00}&{\tt 0.00E+00}&{\tt 15.65}&{\tt 3.36E-02}&{\tt 1.27E-04}&{\tt 9.28E-06}&{\tt 1.29E-03}&{\tt 0.00E+00}\\\hdashline[0.5pt/1pt]
\bench{scalatest}&{\tt 5.29E-05}&{\tt 4.35E-08}&{\tt 1.30E-06}&{\tt 4.41E-06}&{\tt 2.23E-09}&{\tt 20.00}&{\tt 3.71E-02}&{\tt 1.96E-05}&{\tt 5.89E-06}&{\tt 2.65E-04}&{\tt 0.00E+00}\\\hdashline[0.5pt/1pt]
\bench{scalaxb}&{\tt 1.53E-06}&{\tt 0.00E+00}&{\tt 0.00E+00}&{\tt 0.00E+00}&{\tt 0.00E+00}&{\tt 12.42}&{\tt 1.61E-01}&{\tt 3.63E-05}&{\tt 1.21E-06}&{\tt 3.39E-03}&{\tt 0.00E+00}\\\hdashline[0.5pt/1pt]
\bench{specs}&{\tt 8.77E-05}&{\tt 3.16E-09}&{\tt 1.06E-06}&{\tt 7.31E-06}&{\tt 3.93E-09}&{\tt 10.53}&{\tt 4.40E-02}&{\tt 8.04E-05}&{\tt 1.17E-05}&{\tt 6.80E-04}&{\tt 0.00E+00}\\\hdashline[0.5pt/1pt]
\bench{tmt}&{\tt 1.14E-04}&{\tt 4.67E-09}&{\tt 7.31E-11}&{\tt 4.31E-08}&{\tt 4.20E-09}&{\tt 36.54}&{\tt 4.33E+07}&{\tt 1.92E-05}&{\tt 9.72E-08}&{\tt 3.99E-04}&{\tt 0.00E+00}\\
\hline
\multicolumn{12}{c}{\bf SPECjvm2008~\cite{specjvm2008}}\\
\hline
\bench{compiler.compiler}&{\tt 2.36E-06}&{\tt 2.63E-12}&{\tt 5.25E-13}&{\tt 1.37E-11}&{\tt 0.00E+00}&{\tt 98.30}&{\tt 4.39E-02}&{\tt 9.93E-06}&{\tt 1.14E-06}&{\tt 2.42E-04}&{\tt 0.00E+00}\\\hdashline[0.5pt/1pt]
\bench{compiler.sunflow}&{\tt 4.37E-06}&{\tt 2.01E-11}&{\tt 1.32E-13}&{\tt 3.96E-12}&{\tt 0.00E+00}&{\tt 97.85}&{\tt 3.98E-02}&{\tt 8.75E-06}&{\tt 1.48E-06}&{\tt 2.56E-04}&{\tt 0.00E+00}\\\hdashline[0.5pt/1pt]
\bench{compress}&{\tt 3.12E-07}&{\tt 2.02E-12}&{\tt 5.05E-13}&{\tt 2.78E-11}&{\tt 0.00E+00}&{\tt 98.56}&{\tt 4.83E-02}&{\tt 6.31E-10}&{\tt 4.19E-10}&{\tt 4.57E-04}&{\tt 0.00E+00}\\\hdashline[0.5pt/1pt]
\bench{crypto.aes}&{\tt 1.72E-05}&{\tt 2.92E-12}&{\tt 5.85E-13}&{\tt 4.50E-11}&{\tt 0.00E+00}&{\tt 97.63}&{\tt 5.26E-03}&{\tt 7.80E-09}&{\tt 1.07E-08}&{\tt 8.09E-05}&{\tt 0.00E+00}\\\hdashline[0.5pt/1pt]
\bench{crypto.rsa}&{\tt 9.34E-06}&{\tt 9.12E-13}&{\tt 2.28E-13}&{\tt 2.22E-10}&{\tt 0.00E+00}&{\tt 97.33}&{\tt 1.84E-03}&{\tt 5.35E-07}&{\tt 6.67E-07}&{\tt 7.01E-06}&{\tt 3.64E-15}\\\hdashline[0.5pt/1pt]
\bench{crypto.signverify}&{\tt 7.89E-04}&{\tt 1.18E-12}&{\tt 2.95E-13}&{\tt 2.15E-11}&{\tt 0.00E+00}&{\tt 97.65}&{\tt 4.31E-03}&{\tt 1.66E-08}&{\tt 2.74E-08}&{\tt 2.82E-05}&{\tt 0.00E+00}\\\hdashline[0.5pt/1pt]
\bench{derby}&{\tt 1.49E-04}&{\tt 5.07E-09}&{\tt 8.81E-06}&{\tt 6.69E-07}&{\tt 5.08E-12}&{\tt 97.92}&{\tt 3.29E-02}&{\tt 1.29E-05}&{\tt 3.46E-06}&{\tt 1.16E-04}&{\tt 0.00E+00}\\\hdashline[0.5pt/1pt]
\bench{mpegaudio}&{\tt 2.44E-07}&{\tt 2.21E-12}&{\tt 7.81E-14}&{\tt 8.31E-11}&{\tt 0.00E+00}&{\tt 98.29}&{\tt 1.42E-02}&{\tt 3.05E-09}&{\tt 9.78E-08}&{\tt 3.52E-04}&{\tt 2.03E-14}\\\hdashline[0.5pt/1pt]
\bench{scimark.fft.large}&{\tt 2.79E-04}&{\tt 4.99E-12}&{\tt 8.31E-13}&{\tt 3.07E-11}&{\tt 0.00E+00}&{\tt 95.31}&{\tt 4.21E-02}&{\tt 2.55E-09}&{\tt 1.80E-09}&{\tt 2.13E-04}&{\tt 0.00E+00}\\\hdashline[0.5pt/1pt]
\bench{scimark.fft.small}&{\tt 1.25E-03}&{\tt 1.49E-12}&{\tt 3.72E-13}&{\tt 1.34E-11}&{\tt 0.00E+00}&{\tt 98.14}&{\tt 1.41E-01}&{\tt 7.74E-08}&{\tt 8.36E-08}&{\tt 5.31E-04}&{\tt 0.00E+00}\\\hdashline[0.5pt/1pt]
\bench{scimark.lu.large}&{\tt 7.79E-05}&{\tt 2.32E-12}&{\tt 5.80E-13}&{\tt 1.86E-11}&{\tt 0.00E+00}&{\tt 92.28}&{\tt 5.86E-02}&{\tt 9.47E-10}&{\tt 7.28E-10}&{\tt 7.05E-05}&{\tt 0.00E+00}\\\hdashline[0.5pt/1pt]
\bench{scimark.lu.small}&{\tt 1.30E-03}&{\tt 1.30E-12}&{\tt 3.24E-13}&{\tt 1.07E-11}&{\tt 0.00E+00}&{\tt 97.83}&{\tt 1.76E-01}&{\tt 4.85E-08}&{\tt 7.26E-08}&{\tt 3.19E-04}&{\tt 0.00E+00}\\\hdashline[0.5pt/1pt]
\bench{scimark.sor.large}&{\tt 2.14E-04}&{\tt 2.12E-12}&{\tt 4.24E-13}&{\tt 1.65E-11}&{\tt 0.00E+00}&{\tt 92.38}&{\tt 6.86E-02}&{\tt 1.67E-09}&{\tt 1.05E-09}&{\tt 1.58E-04}&{\tt 0.00E+00}\\\hdashline[0.5pt/1pt]
\bench{scimark.sor.small}&{\tt 2.20E-04}&{\tt 1.83E-12}&{\tt 3.66E-13}&{\tt 1.43E-11}&{\tt 0.00E+00}&{\tt 98.22}&{\tt 2.75E-02}&{\tt 2.25E-08}&{\tt 1.65E-08}&{\tt 1.93E-04}&{\tt 0.00E+00}\\\hdashline[0.5pt/1pt]
\bench{scimark.sparse.large}&{\tt 2.65E-04}&{\tt 3.16E-12}&{\tt 7.90E-13}&{\tt 2.53E-11}&{\tt 0.00E+00}&{\tt 87.15}&{\tt 1.27E-01}&{\tt 2.07E-09}&{\tt 1.54E-09}&{\tt 1.91E-04}&{\tt 0.00E+00}\\\hdashline[0.5pt/1pt]
\bench{scimark.sparse.small}&{\tt 1.66E-04}&{\tt 3.47E-12}&{\tt 6.93E-13}&{\tt 2.22E-11}&{\tt 0.00E+00}&{\tt 96.42}&{\tt 7.21E-02}&{\tt 3.49E-08}&{\tt 4.93E-08}&{\tt 3.55E-04}&{\tt 0.00E+00}\\\hdashline[0.5pt/1pt]
\bench{serial}&{\tt 7.14E-04}&{\tt 6.99E-11}&{\tt 2.38E-11}&{\tt 2.65E-10}&{\tt 0.00E+00}&{\tt 98.09}&{\tt 1.16E-02}&{\tt 1.14E-05}&{\tt 6.74E-06}&{\tt 2.37E-04}&{\tt 6.43E-15}\\\hdashline[0.5pt/1pt]
\bench{sunflow}&{\tt 4.38E-09}&{\tt 1.91E-11}&{\tt 4.25E-14}&{\tt 2.19E-11}&{\tt 0.00E+00}&{\tt 96.95}&{\tt 1.26E-02}&{\tt 2.17E-05}&{\tt 5.36E-07}&{\tt 5.34E-04}&{\tt 0.00E+00}\\\hdashline[0.5pt/1pt]
\bench{xml.transform}&{\tt 2.43E-04}&{\tt 3.58E-12}&{\tt 5.12E-13}&{\tt 1.23E-11}&{\tt 0.00E+00}&{\tt 97.82}&{\tt 1.16E-02}&{\tt 8.05E-06}&{\tt 3.56E-06}&{\tt 3.56E-04}&{\tt 0.00E+00}\\\hdashline[0.5pt/1pt]
\bench{xml.validation}&{\tt 2.33E-04}&{\tt 1.30E-12}&{\tt 2.59E-13}&{\tt 3.16E-11}&{\tt 0.00E+00}&{\tt 98.80}&{\tt 2.38E-02}&{\tt 7.80E-06}&{\tt 3.00E-06}&{\tt 3.43E-04}&{\tt 0.00E+00}\\
\hline
\end{tabular}
